# Supplementary material for: CIMI4D: A Large Multimodal Climbing Motion Dataset under Human-scene Interactions
Source: arXiv:2303.17948 source file (2023-03-31)
Supplement: Supplementary file 1 [file appendix.tex]

\section{Appendix}\label{secs:appendix}

\subsection{Coordinates}

\PAR{Coordinate Systems.} 
We define three coordinate systems: 1) IMU coordinate system \{$I$\}: origin is at the pelvis joint of the first SMPL model, and $X/Y/Z$ axis is pointing to the right/upward/forward of the human. 2) LiDAR Coordinate system \{$L$\}: origin is at the center of the LiDAR, and $X/Y/Z$ axis is pointing to the right/forward/upward of the LiDAR. 3) Global/World coordinate system \{$W$\}: the scene's coordinate we manually define. We use the right subscript $k, k\in~Z^+$ to indicate the index of a frame, and the right superscript, $I$ or $L$ or $W$ (default to $W$), to indicate the coordinate system that the data belongs to. For example, the 3D point cloud frames from LiDAR is represented as $P^L = \{P_k^L, k\in~Z^+\}$

\PAR{Coarse calibration.}Before data capturing, the actor stands facing or parallel to a large real-world object with a flat face, such as a wall or a square column. His right/front/up is regarded as the scene's $X/Y/Z$ axis direction, and the midpoint of his ankles' projection on the ground is set as the origin. After the data are collected, we manually find the first frame's ground plane and the object's plane, and then calculate their normal vector $g=[g_1,g_2,g_3]^\top$ and $m=[m_1, m_2, m_3]^\top$, respectively. The coarse calibration matrix $R_{WL}$ from the LiDAR starting position to the world coordinate \{$W$\} is calculated as:
\begin{equation}
R_{WL} = \begin{bmatrix}
e_1 & e_2 & e_3 & 0\\
m_1 & m_2 & m_3 & 0.2\\
g_1 & g_2 & g_3 & h \\
0   & 0   & 0   & 1
\end{bmatrix}
\end{equation} where $[e_1, e_2, e_3]^\top = m \times g$ and $h$ is the height of the LiDAR from the ground.
Based on the definition of IMU coordinate system \{$I$\}, the coarse calibration matrix $R_{WI}$ from \{$I$\} to \{$W$\} is defined as:
$R_{WI}= \begin{bmatrix}(1,1,-1)(2,3,1)(3,2,1)(4,4,1)\end{bmatrix}_{triad}$

We use the right subscript $k, k\in~Z^+$ to indicate the index of a frame, and the right superscript, $I$ or $L$ or $W$ (default to $W$), to indicate the coordinate system that the data belongs to. For example, the 3D point cloud frames from LiDAR is represented as $P^L = \{P_k^L, k\in~Z^+\}$ and the 3D scene is represented as \bm{$S$}. $M_k^W$ indicates the $k$-th frame in human motion $M=(T, \theta, \beta)$ in world coordinate system, where $T$ is the $N\times3$ translation parameter, $\theta$ is the $N\times24\times3$ pose parameter, and $\beta$ is the $N\times10$ shape parameter. We use the Skinned Multi-Person Linear (SMPL)~\cite{SMPL2015} body model $\varPhi$ to map $k$-th frame's motion representation $M_k$ to its triangle mesh model, $V_k, F_k =\varPhi(M_k)$, where body vertices $V_k\in~\mathbb{R}^{6890\times3}$ and faces $F_k\in~\mathbb{R}^{13690\times3}$.

We first obtain the 3D human motion output by the inertial MoCap system. Then we estimate the self-motion of LiDAR and build a 3D scene map \bm{${S}$} through point cloud data $P_k^I$. Finally, based on the coarse calibration and synchronization result, we perform a data initialization to prepare data for further optimization. 

%3.4. Blend Optimization Stage

\PAR{Limb contact Loss.} This loss is defined as the distance from a stable foot or hand to its nearest neighbor in the scene vertices. First, we detect the foot and hand state based on its movements. The movement is calculated based on the set of vertices of hands ${VF}_k$ and feet ${VH}_k$ for frame $k$. One limb is marked as stable if its movement is smaller than 3$cm$ and smaller than another limb (foot or hand)'s movement. We obtain the contact environment $pf_k$ and $ph_k$ near the stable limb through a neighbor search. The limb contact loss $\mathcal{L}_{ct} = \mathcal{L}_{\text {ct}_{feet}} + \mathcal{L}_{\text {ct}_{hand}}$ is written as:
%\begin{equation}
%	\begin{split}
%        \mathcal{L}_{\text {ct}_{feet}}=\frac{1}{l}{
%        \sum_{j=k}^{k+l}
%        \sum_{v \in VF^{\mathcal{SF}_j}}
%        \frac{1}{|VF^{\mathcal{SF}_j}|}\|v-\widetilde{v} \cdot pf_j\|_{2}}
%    \end{split}
%    \label{equ:cont}
%\end{equation}

%\begin{equation}
%	\begin{split}
%       \mathcal{L}_{\text {ct}_{hand}}=\frac{1}{l}{
%        \sum_{i=k}^{k+l}
%        \sum_{v \in VH^{\mathcal{SH}_j}}
%        \frac{1}{|VH^{\mathcal{SH}_j}|}\|v-\widetilde{v \cdot ph_i\|_{2}}
%    \end{split}
%    \label{equ:cont}
%\end{equation}

\begin{equation}
	\begin{split}
        \mathcal{L}_{\text {ct}_{feet}}= \frac{1}{l}\sum_{j=1}^{l-1}
        \sum_{v \in VF^{\mathcal{SF}_j}}
        \frac{1}{|VF^{\mathcal{SF}_j}|}\|v-\widetilde{v} \cdot pf_j\|_{2}
    \end{split}
    \label{equ:cont}
\end{equation}
\begin{equation}
\begin{split}
        \mathcal{L}_{\text {ct}_{hand}}= \frac{1}{l}\sum_{j=1}^{l-1}
        \sum_{v \in VH^{\mathcal{SH}_j}}
        \frac{1}{|VH^{\mathcal{SH}_j}|}\|v-\widetilde{v} \cdot ph_j\|_{2}
        \end{split}
    \label{equ:cont}
\end{equation}
\noindent
where $\widetilde{v_{f}}$ and $\widetilde{v_{h}}$ is homogeneous coordinate of $v_f$ and $v_h$. $VF^{\mathcal{SF}_j}$ and $VH^{\mathcal{SH}_i}$ are the sets of the vertices of a stable foot $\mathcal{SF}_j$  and a stable hand $\mathcal{SH}_i$. The loss is average over all frames of a sequence with length $l$.  %$VF_j=\varPhi(\bm{M}_j, V_{feet})$ and $VH_i=\varPhi(\bm{M}_i, V_{hands})$.

\PAR{Limb sliding Loss.} This loss reduces the motion's sliding on the contact surfaces, making the motion more natural and smooth. The sliding loss: $\mathcal{L}_{sld} = \mathcal{L}_{\text {sld}_{feet}} + \mathcal{L}_{\text {sld}_{hands}}$ is defined as every two successive stable limb's distance.
\begin{equation}
	\begin{split}
        \mathcal{L}_{\text {sld}_{feet}}= \frac{1}{l}\sum_{j=1}^{l-1}
        \|\mathbb{E}{(VF^{\mathcal{SF}_{j+1}})}-\mathbb{E}(VF^{\mathcal{SF}_{j}})\|_{2}
    \end{split}
    \label{equ:sld}
\end{equation}
\vspace{-2mm} 
\begin{equation}
	\begin{split}
        \mathcal{L}_{\text {sld}_{hands}} = \frac{1}{l}\sum_{j=1}^{l-1}
        \|\mathbb{E}{(VH^{\mathcal{SH}_{j+1}})}-\mathbb{E}(VH^{\mathcal{SH}_{j}})\|_{2}
    \end{split}
    \label{equ:sld}
\end{equation}
\noindent where $\mathbb{E}(\cdot )$ calculates the center of the vertices list.

\PAR{Smooth Loss.} The smooth loss includes the translation term $\mathcal{L}_{trans}$ and the joints term $\mathcal{L}_{joints}$. 
\begin{equation}
	\begin{split}
        \mathcal{L}_{smt} = 
        \lambda_{trans} \mathcal{L}_{trans} + 
        \lambda_{joints} \mathcal{L}_{joints}
    \end{split}
\end{equation}
The $\mathcal{L}_{trans}$ smooths the trajectory $T$ of human (the translation of the pelvis) through minimizing the difference between LiDAR and a human's translation difference. The smooth term is as follows: 
\vspace{-2mm} 
\begin{equation}
	\begin{split}
	\mathcal{L}_{trans} = \frac{1}{l}\sum_{j=1}^{l-1}{\max(0, \|T_{j+1}^L - T_{j}^L\|_2 - \|T_{j+1} - T_{j}\|_2)}
    \end{split}
\end{equation}
\noindent where $T_{k}^L$ is the translation of LiDAR at $k$-th frame, and $T_{k}$ is the translation we optimized for.

The $\mathcal{L}_{joints}$ is the term that smooths the motion of body joints in global 3D space, which minimizes the mean acceleration of the joints. For this loss, we only choose stable joints $J^s$, i.e., the joints on the torso and the neck. Let $\delta^s_j = J^s_j-J^s_{j-1}$ represent the difference of joints between consecutive frame. $\mathcal{L}_{joints}$ is defined as follows.
\vspace{-2mm} 
\begin{align}
    \mathcal{L}_{joints}=
    \frac{1}{l}
   \sum_{j=1}^{l-1} 
    \|\delta^s_{j+1} - \delta^s_j\|_{2}
\end{align}
%\begin{equation}
%    \mathcal{L}_{joints}=\frac{1}{l}
%    \sum_{j=k}^{k+l-1} 
%    \|J_{stable}{(V_{j+1})}-J_{stable}(V_{j})\|_{2}
%\end{equation}

%Since the static scenes are collected in~\cref{sec:Hardware}, we design a method to segment human point clouds as annotation data. For each frame of dynamic LiDAR output, we manually register to the same coordinate system of the IMU to obtain the RT matrix. Next, the human body in the multi-frame dynamic scene is manually removed to generate a sparse static scene. For each frame of point cloud, the points within the threshold range of the sparse scene are eliminated to obtain the segmented human point cloud $\mathcal{P}_i$.
%For each segmented human point cloud $\mathcal{P}_i$.
\PAR{Mesh to point loss.} %
For each estimated human meshes, we use Hidden Points Removal (HPR) \cite{katz2007direct} to remove the invisible mesh vertices from the perspective of LiDAR. Then, we use Iterative closest point (ICP)~\cite{segal2009generalized} to register the visible vertices to $\mathcal{P}$, which is segmented human point clouds. We re-project the human body mesh in the LiDAR coordinate to select the visible human body vertices $V'\,\!$. We use $\mathcal{L}_{m2p}$ to minimize the 3D Chamfer distance of human points $\mathcal{P}_{i}$ and $V'\,\!_{i}$. For each frame, the $\mathcal{L}_{m2p}$ constraint is regularized with the following equation: 
\begin{equation}
    {{\mathcal{L}}_{m2p}}=
    \frac{1}{|\mathcal{P}|}\sum\limits_{{{p}_{i}}\in \mathcal{P}}
    {\underset{{{v}_{i}}\in {V}'}{\mathop{\min }}
    \,\left\| {{p}_{i}}-{{v}_{i}} \right\|_{2}^{2}+}
    \frac{1}{|{V}'|}\sum\limits_{{{v}_{i}}\in {V}'}{\underset{{{p}_{i}}\in \mathcal{P}}{\mathop{\min }}\,\left\| {{v}_{i}}-{{p}_{i}} \right\|_{2}^{2}}
\end{equation}
